# Supplementary material for: Ultrasensitive strain modulation of terahertz magnons at a magnetic phase transition
Source: arXiv:2602.13924 ancillary file (2026-02-14)
Supplement: Supplementary file 1 [file supplementary_information.pdf]

# Supplementary information for "ultrasensitive strain modulation of terahertz magnons at a magnetic phase transition"

Lichen Wang,[1,*] Sajna Hameed,[1] Yiran Liu,[1] Manuel Knauft,[1] Kazuki Higuchi,[1] Maximilian Krautloher,[1] Sonia Francoual,[2] Giniyat Khaliullin,[1] Huimei Liu,[1,3,4,†] Matteo Minola,[1,‡] and Bernhard Keimer[1,§]

[1]*Max Planck Institute for Solid State Research, Heisenbergstrasse 1, D-70569 Stuttgart, Germany*
[2]*Deutsches Elektronen-Synchrotron DESY, Notkestrasse 85, D-22607 Hamburg, Germany*
[3]*National Laboratory of Solid State Microstructures and School of Physics, Nanjing University, Nanjing 210093, China*
[4]*Collaborative Innovation Center of Advanced Microstructures, Nanjing University, Nanjing 210093, China*

(Dated: February 13, 2026)

## CONTENTS

I. Supplementary Note 1: Sample Information and Strain Calibration 1

II. Supplementary Note 2: Additional Raman and RXD data 3

III. Supplementary Note 3: Additional information on theoretical model 8
A. Spin-orbital levels and magnetic anisotropy 8
B. Interlayer coupling and magnetic phase transition 9

References 11

## I. Supplementary Note 1: Sample Information and Strain Calibration

**Supplementary Table 1**. **Sample dimensions and experiment information of $Ca_2RuO_4$ under uniaxial strain.** Single crystals were cut into needle-like shapes with the $c-$axis oriented along the surface normal. Uniaxial strain was applied along the long dimension of each specimen. **Length** denotes the strained direction; **Width** indicates the in-plane direction perpendicular to strain; **Thickness** refers to out-of-plane dimension along the $c-$axis.

| Sample | Strain | Length ($\mu$m) | Width ($\mu$m) | Thickness ($\mu$m) | Exp. |
|---|---|---|---|---|---|
| A | [1 0 0] | 600 | 200 | 100 | Raman |
| B | [1 0 0] | 420 | 180 | 90 | Raman |
| C | [1 1 0] | 600 | 210 | 100 | Raman, RXD |
| D | [1 1 0] | 600 | 200 | 60 | Raman |
| E | [1 1 0] | 650 | 250 | 110 | RXD |

The needle-like specimen is subjected to uniaxial strain via voltages applied to piezoelectric actuators. Owing to the incomplete transmission of the device displacement through the epoxy medium to the crystal, the actual strain values are determined from lattice parameters measured by X-ray diffraction. Since in-situ diffraction measurements within the Raman setup are not feasible, we calibrated the strain values prior to the Raman experiments by performing X-ray diffraction on the same sample at a similar temperature.

The calibration of strain along the [1 0 0] direction is presented in Supplementary Fig. 1. The (2 0 0) Bragg reflection was measured at 20 K using a transmission scattering geometry on our in-house diffractometer, directly probing the lattice constant along the strain direction. Here, the Mo $K\alpha$ emission line ($\sim$ 17.45 keV) was used without removing the $K\alpha_2$ satellite line, resulting in weak shoulder peaks as shown in Supplementary Fig. 1a. Despite this, the diffraction scans exhibits clear and systematic shifts under compression, and the strain response is reversible upon its release, confirming elastic deformation of the strained sample. Quantitative analysis in Supplementary Fig. 1b

* lichen.wang@fkf.mpg.de
† huimeiliu@nju.edu.cn
‡ m.minola@fkf.mpg.de
§ b.keimer@fkf.mpg.de

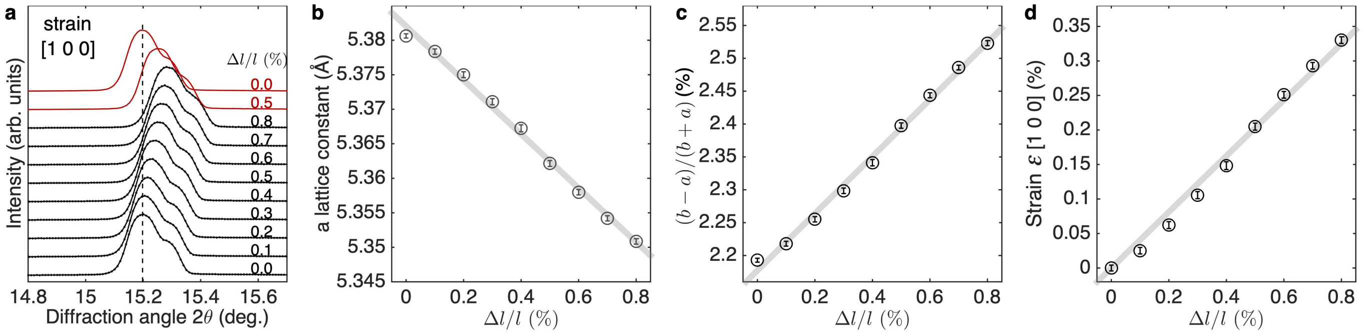


**Supplementary Figure 1**. **Calibration of strain along the [1 0 0] direction using laboratory x-ray diffraction. a**, At around 20 K, $\theta-2\theta$ scans of the (2 0 0) Bragg reflection with increasing (black curves) and releasing (red curves) compression along the [1 0 0] direction. The positive value of $\Delta l/l$ coresponds to compression. **b**, Lattice constant $a$ obtained from the (2 0 0) Bragg reflections as a function of $\Delta l/l$. **c-d**, Orthorhombicity $(b-a)/(b+a)$ and strain $\varepsilon$. The grey lines in all panels are linear fits to the data.

shows a linear response of the lattice constant $a$ to the normalized displacement of the strain device $\Delta l/l$, where $\Delta l$ is the displacement of piezoelectric stacks and $l$ the strained sample length. Here, $\Delta l$ is monitored using an ultra-high-sensitivity capacitance bridge and is precisely controlled via the input voltage, enabling the quantitative application of uniaxial strain.

The in-plane strain directly modifies the lattice orthorhombicity, thereby tuning the magnetic anisotropy via pseudospin-lattice coupling. Accordingly, the strain value is defined as the relative change in lattice orthorhombicity for theoretical modeling of the magnetic response. For strain-free $Ca_2RuO_4$, the intrinsic orthorhombicity $\varepsilon_0 = (b_0 - a_0)/(b_0 + a_0)$ is 2.2%, with $a_0$ = 5.382 Å and $b_0$ = 5.622 Å measured at 20 K (space group *Pbca*). Under compressive strain along the shorter [1 0 0] axis, the lattice orthorhombicity increases, as shown in Supplementary Fig. 1(c). The induced strain $\varepsilon$ is defined as $|(b-a)/(b+a) - \varepsilon_0|$, where $a$ and $b$ are lattice constants under strain. To determine $\varepsilon$, the in-plane Poisson ratio $\nu = 0.2$ for $Ca_2RuO_4$ [1] is used to estimate the lattice constant $b$, which is not directly measurable in our strain setup. The uncertainties in both orthorhombicity and $\varepsilon$ are propagated from the errors in the lattice constants—a procedure applied to both strain directions. Supplementary Fig.1 reveals a linear relationship between $\varepsilon$ and $\Delta l/l$. This established scaling factor was subsequently used to estimate the strain levels during the Raman measurements.

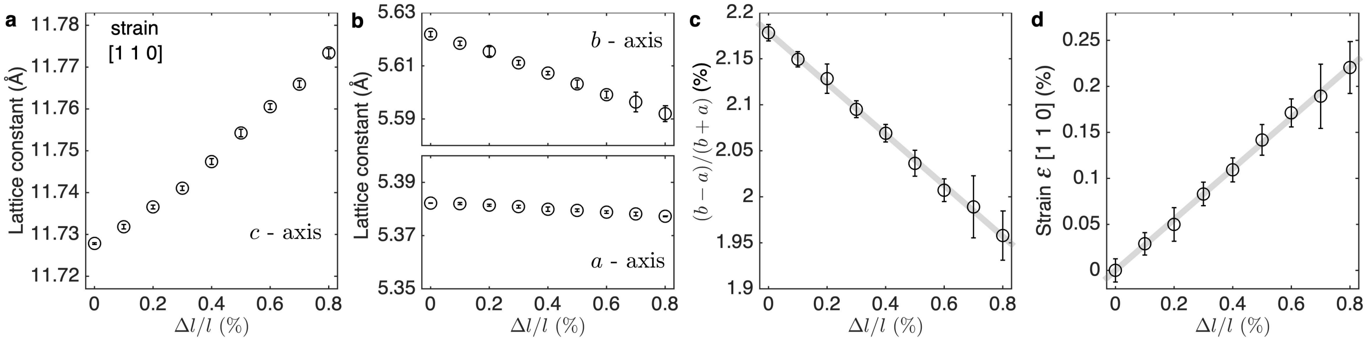


**Supplementary Figure 2**. **Calibration of strain along the [1 1 0] direction using RXD. a-b**, At around 20 K, lattice constants $a$, $b$ and $c$ obtained from Bragg reflections under compression along the [1 1 0] direction. Under compression, $c$-axis expands while $a$ and $b$ decreases. **c-d**, Orthorhombicity $(b-a)/(b+a)$ and strain $\varepsilon$ calculated from the panel (**b**). The grey lines are linear fits to data. The positive values of $\Delta l/l$ and $\varepsilon$ correspond to compression. The magnetic phase transition occurs at $\Delta l/l \sim 0.5\%$ ($\varepsilon \sim 0.15\%$).

The strain along the [1 1 0] direction was calibrated during measurements of magnetic reflections at the Ru $L_3$ edge ($\sim$ 2.8 keV), using a reflection scattering geometry at the P09 beamline at PETRA-III (DESY). The strain $\varepsilon$ along this direction is defined in the same manner as above, retaining the convention that a positive value of strain denotes compression. Although compression along the [1 1 0] direction induces a shear distortion relative to the orthorhombic

axes, the substantial orthorhombicity of $Ca_2RuO_4$ justifies that $\varepsilon$ is still defined using the orthorhombic axes within the small strain regime. Here, multiple Bragg reflections including (0 0 4), (1 0 4) and (1 -1 3) were measured to determine the lattice constants $a$, $b$ and $c$. Supplementary Fig. **2** shows a pronounced decrease in $b$ accompanied by a subtle reduction in $a$, revealing that compressive strain along the [1 1 0] direction monotonically reduces the lattice orthorhombicity up to $\varepsilon \sim 0.22$ %. Likewise, a scaling factor between $\varepsilon$ and $\Delta l/l$ was obtained for strain calibration.

The application of uniaxial strain induces the B-centered AFM phase in a structure characterized by reduced lattice orthorhombocity and an expanded $c$-axis, consistent with earlier studies of this magnetic transition being achieved via chemical doping [2–6] or pressure [7]. Quantitative comparison with literature reveals that a small critical strain $\varepsilon \sim 0.15\%$ is sufficient to stabilize the B-centered phase, requiring significantly smaller structural modifications than previously reported (see Supplementary Table **2**; only the published data taken at similar temperatures near 20 K are listed for comparison). Additionally, previous studies indicate that the ordered magnetic moments in the B-centered phase remain aligned along the $b$-axis [2–5, 7] even under substantially reduced orthorhombicity, *e.g.* $\sim 0.6\%$ in the Sr-doped sample [5], compared to the orthorhombicity of $\sim 2.0\%$ in the present study. Therefore, we assume that the spin easy-axis remains its $b$-axis orientation under strain throughout the transition into the B-centered phase.

**Supplementary Table 2**. Available structural information at around 20 K for A- and B-centered AFM phases from our measurements and wide literature, including lattice constants and orthorhombicity $\frac{b-a}{b+a}$.

| Compound | $Ca_2RuO_4$ (this work, [2]) | $Ca_2RuO_4$ [1 1 0] strain (this work) | $Ca_2Ru_{0.88}Fe_{0.12}O_4$ [3] | $Ca_{1.95}La_{0.05}RuO_4$ [4] | $Ca_2RuO_4$ hydrostatic 0.3 GPa [7] | $Ca_2RuO_{4.07}$ [2] | $Ca_{1.9}Sr_{0.1}RuO_4$ [5] |
|---|---|---|---|---|---|---|---|
| $a$ (Å) | **5.382** | **5.380** | 5.405 | 5.387 | 5.390 | 5.407 | 5.421 |
| $b$ (Å) | **5.622** | **5.603** | 5.595 | 5.573 | 5.560 | 5.515 | 5.480 |
| $c$ (Å) | **11.728** | **11.754** | 11.763 | 11.833 | n.a. | 11.905 | 11.940 |
| $\frac{b-a}{b+a}$ (%) | **2.2** | **2.0** | 1.7 | 1.7 | 1.6 | 1.0 | 0.6 |

## II. Supplementary Note 2: Additional Raman and RXD data

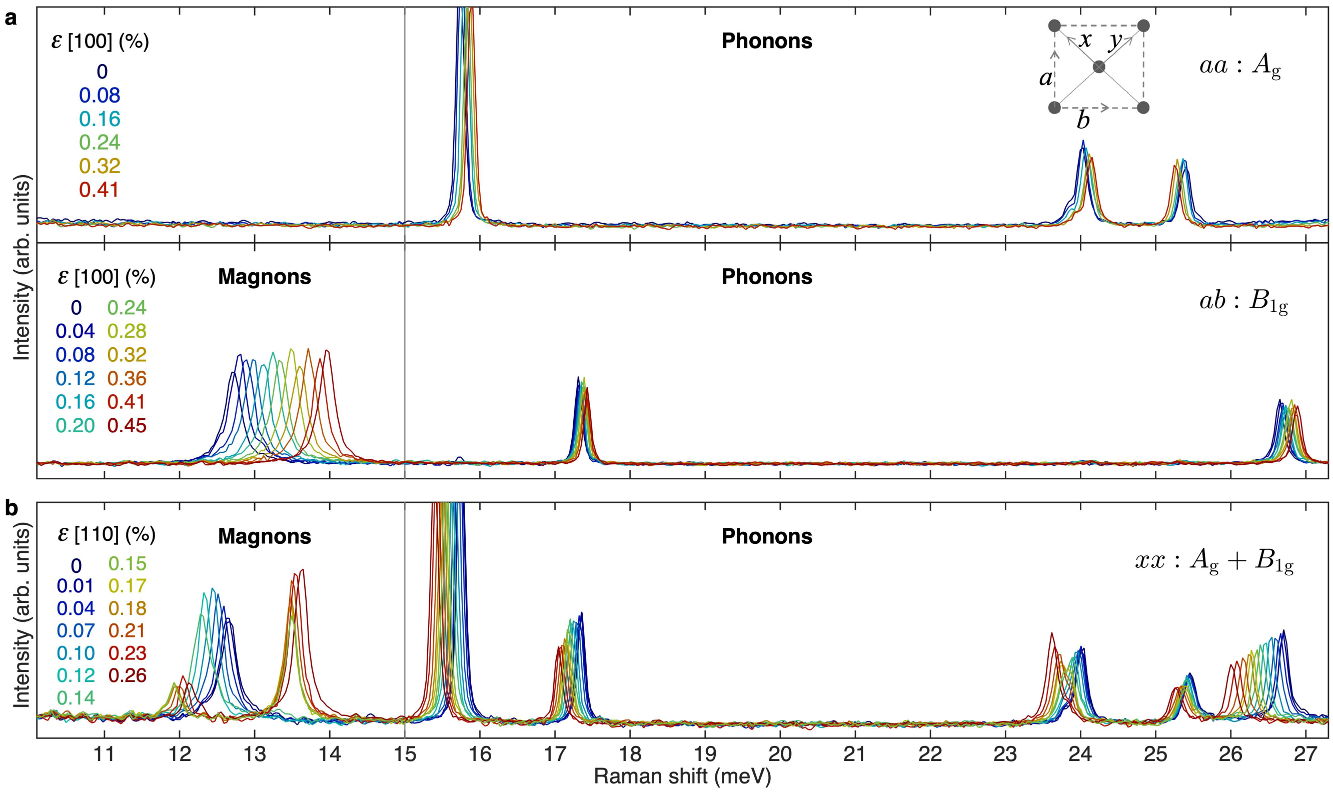


**Supplementary Figure 3**. **Low-temperature Raman spectra under compressive strain along the [1 0 0] and [1 1 0] directions over an extended energy range.** **a**, Spectra in the $A_{\mathrm{g}}$ (upper panel) and $B_{1\mathrm{g}}$ (middle panel) channels, measured using parallel ($aa$) and cross ($ab$) linear polarization configurations respectively. The inset shows Ru-lattice structure with the $x/y$-axis corresponding to the [1 1 0] direction and $a(b)$-axis corresponding to the [1 0 0]([0 1 0]) direction. **b**, In this setup, the linear polarization of incident photons is fixed along the strain ([1 1 0]) direction, i.e. $x$-axis. The parallel polarization channel ($xx$) contains contributions from both $A_{\mathrm{g}}$ and $B_{1\mathrm{g}}$ symmetries, while the cross polarization channel ($xy$) detects no Raman features (Supplementary Fig. 5). Despite this, the magnon features below 14 meV remain clearly distinguishable from phonons by their distinct energy scales.

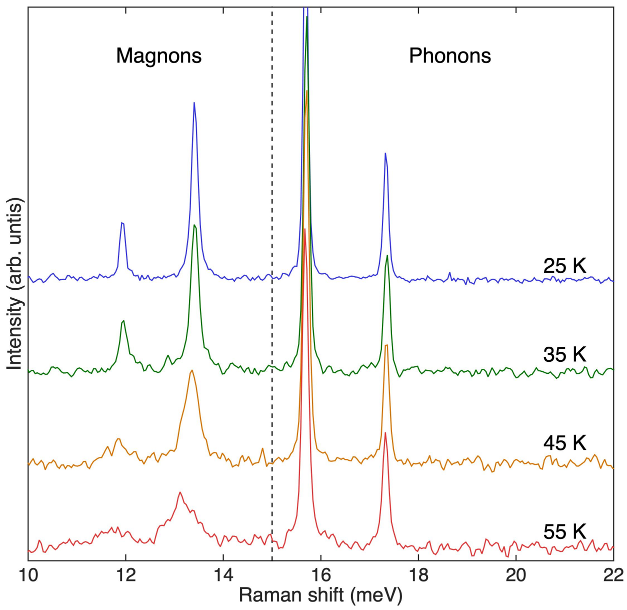


**Supplementary Figure 4**. **Temperature-dependent Raman spectra under compressive [1 1 0] strain $\varepsilon \sim$ 0.17%.**

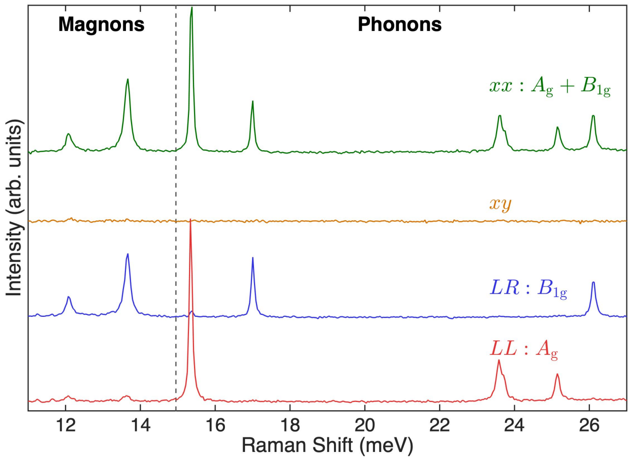


**Supplementary Figure 5**. **Raman spectra under compressive [1 1 0] strain $\varepsilon \sim$ 0.26% measured with circular polarizations.** Spectra with four different polarization configurations at around 25 K. Using co-circular ($LL$) and cross-circular ($LR$) polarization configurations, the $A_g$ and $B_{1g}$ channels are clearly separated, confirming magnon features below 15 meV in the $B_{1g}$ channel.

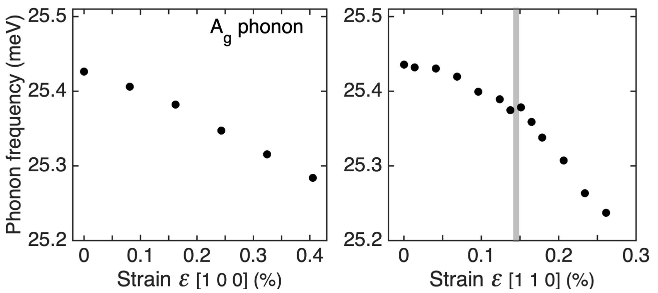


**Supplementary Figure 6**. **Frequencies of the $A_{\mathrm{g}}$ phonon mode near 25.4 meV under compressive strains along the [1 0 0] (left) and [1 1 0] (right) directions.** The frequencies were extracted from Lorentzian fits to the Raman spectra. The vertical line in the right panel indicates the critical strain $\varepsilon \sim 0.15\%$, where the magnetic phase transition alters the strain dependence of the phonon frequency.

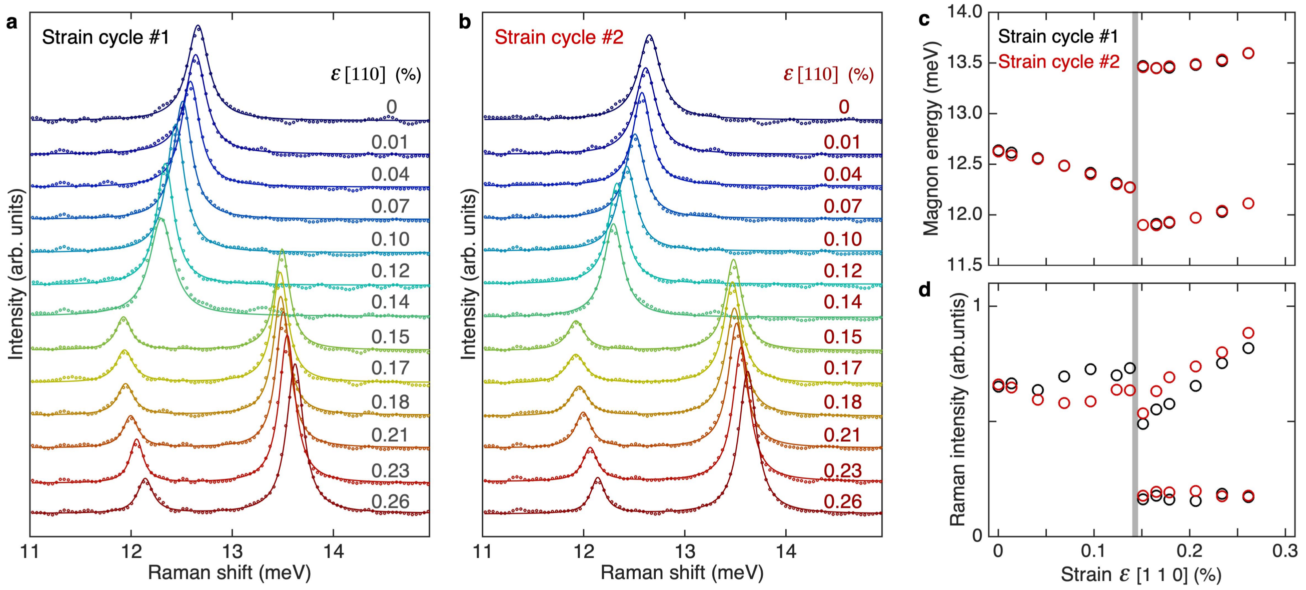


**Supplementary Figure 7**. **Raman spectra under compressive strain along the [1 1 0] direction across multiple strain cycles. a-b**, Spectra taken at the same sample spot over two successive strain cycles. The strain-induced magnon modifications are reversible and reproducible, occurring at nearly identical critical strains. **c-d**, The fitting results for the magnon energy and intensity are consistent across different cycles.

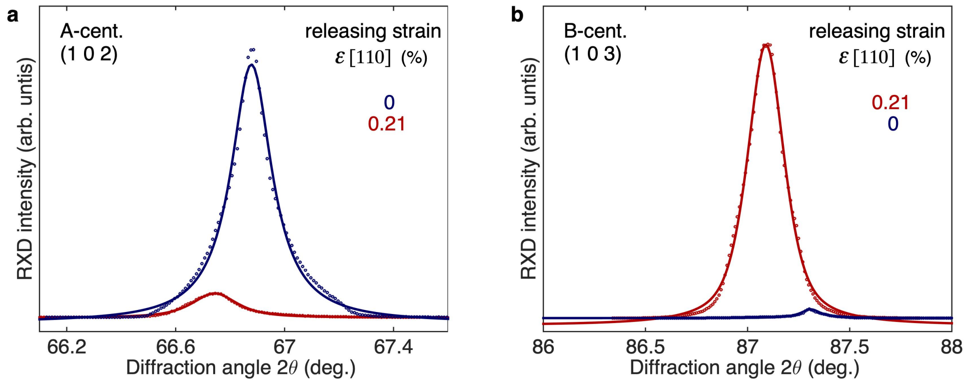


**Supplementary Figure 8**. **Magnetic reflections upon the release of the compressive strain along the [1 1 0] strain.** The recovery of the reflections demonstrates the reversibility of the magnetic response.

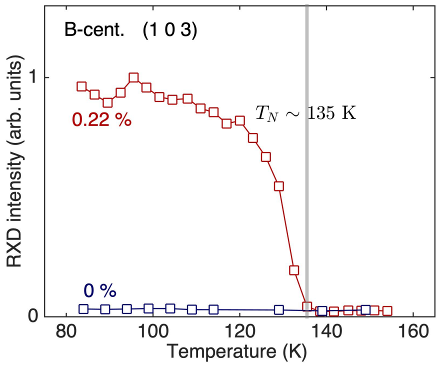


**Supplementary Figure 9**. **Temperature-dependent RXD intensity of the magnetic reflection for the B-centered phase.** Intensity of the (1 0 3) reflection at the Ru-$L_3$ edge under [1 1 0] compressive strains $\varepsilon \sim 0\%$ (blue) and 0.22% (red). The strain-stabilized B-centered phase exhibits a Néel temperature $T_\mathrm{N} \sim 135$ K (vertical line), higher than that of the A-centered phase in unstrained crystals.

## III. Supplementary Note 3: Additional information on theoretical model

### A. Spin-orbital levels and magnetic anisotropy

The electronic configuration of $Ru^{4+}$ in $Ca_2RuO_4$ is $d^4$, and its low-spin state can be described with $s = 1, l = 1$ with $l$ being the effective orbital angular momentum describing 3-fold orbital degeneracy. The single-ion anisotropy Hamiltonian including spin-orbit coupling and tetragonal crystal field is written as:

$$\mathcal{H} = \lambda \boldsymbol{l} \cdot \boldsymbol{s} + \Delta(l_z^2 - \tfrac{2}{3}) \ . \tag{S1}$$

Diagonalization of this Hamiltonian results in the spin-orbital levels shown in Supplementary Fig. 10a. In the $|l_z, s_z\rangle$ basis, the ground-state singlet $|s\rangle$ reads as:

$$|s\rangle = \sin\theta_0 \tfrac{1}{\sqrt{2}}(|1,-1\rangle + |-1,1\rangle) - \cos\theta_0 |0,0\rangle \ . \tag{S2}$$

The triplet states $T_a = \frac{1-i}{2}\ T_1 + \frac{1+i}{2}\ T_{-1}$, $T_b = \frac{1+i}{2} T_1 + \frac{1-i}{2} T_{-1}$ and $T_z = iT_0$ are given by:

$$\begin{aligned} |T_{+1}\rangle &= \cos\theta_1 |0,1\rangle - \sin\theta_1 |1,0\rangle \ , \\ |T_{-1}\rangle &= \sin\theta_1 |-1,0\rangle - \cos\theta_1 |0,-1\rangle \ , \\ |T_0\rangle &= \tfrac{1}{\sqrt{2}}(|-1,1\rangle - |1,-1\rangle) \ . \end{aligned} \tag{S3}$$

For completeness, we also show wave functions of the high-energy quintuplet $\tilde{J} = 2$ states:

$$\begin{aligned} |Q_{\pm 2}\rangle &= |\pm 1, \pm 1\rangle \ , \\ |Q_{\pm 1}\rangle &= \sin\theta_1 |0,\pm 1\rangle + \cos\theta_1 |\pm 1, 0\rangle \ , \\ |Q_0\rangle &= \cos\theta_0 \tfrac{1}{\sqrt{2}}(|1,-1\rangle + |-1,1\rangle) + \sin\theta_0 |0,0\rangle \ . \end{aligned} \tag{S4}$$

Here the spin-orbit mixing angles are:

$$\tan\theta_0 = \frac{1}{\sqrt{2}}\big(\sqrt{\tfrac{9}{4} - \delta + \delta^2} - \delta + \tfrac{1}{2}\big) \ , \qquad \tan\theta_1 = \frac{2\lambda}{\Delta + \sqrt{4\lambda^2 + \Delta^2}} \ , \tag{S5}$$

with $\delta = \frac{\Delta}{2\lambda}$.

The energies of the above spin-orbital levels are:

$$\begin{aligned} E_s &= -\sqrt{2}\lambda \tan\theta_0 - \tfrac{2}{3}\Delta \ , \\ E_{T_{a/b}} &= -\lambda \tan\theta_1 - \tfrac{2}{3}\Delta \ , \\ E_{T_z} &= -\lambda + \tfrac{1}{3}\Delta \ , \\ E_{Q_{\pm 2}} &= \lambda + \tfrac{1}{3}\Delta \ , \\ E_{Q_{\pm 1}} &= \frac{\lambda}{\tan\theta_1} - \tfrac{2}{3}\Delta \ , \\ E_{Q_0} &= \lambda(\sqrt{2}\tan\theta_0 - 1) + \tfrac{1}{3}\Delta \ . \end{aligned} \tag{S6}$$

The first excited doublet level $T_{a/b}$ has the excitation energy:

$$E = E_{T_{a/b}} - E_s = \lambda\big(\tfrac{1}{2} + \sqrt{\tfrac{9}{4} - \delta + \delta^2} - \sqrt{1 + \delta^2}\big) \ . \tag{S7}$$

Under the orthorhombic crystal field $\frac{1}{2}\Delta_{\text{ort}}(n_{az} - n_{bz})$, the $T_{a/b}$ doublet is split by:

$$\kappa = \frac{1}{2}\left(1 - \frac{\delta}{\sqrt{1+\delta^2}}\right)\Delta_{\text{ort}} \ , \tag{S8}$$

as shown in Supplementary Fig. 10b.

In the strong SOC limit of $\delta \to 0$, the orbital moment is unquenched, single-ion anisotropy can be as large as $\kappa = \frac{1}{2}\Delta_{\text{ort}}$, generating a large magnon gap. At large $\Delta$, orbital moment is quenched and the in-plane anisotropy reduces to $\kappa \simeq (\lambda/\Delta)^2 \cdot \Delta_{\text{ort}}$. A monotonic reduction of $\kappa$ with increased $\Delta$ is shown in Supplementary Fig. 11.

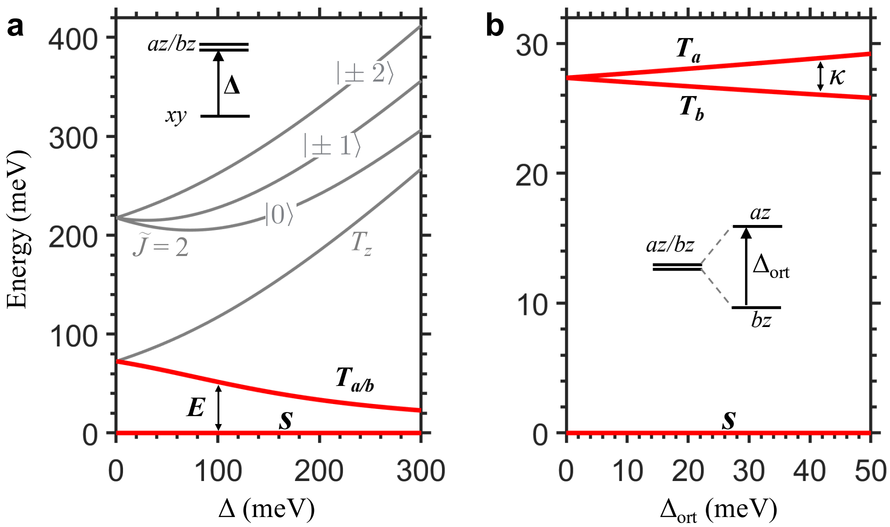


**Supplementary Figure 10**. **Spin-orbital levels under tetragonal $\Delta$ and orthorhombic $\Delta_{\rm ort}$ crystal fields.** **a,** Energy splitting of $s = 1, l = 1$ manifold under spin-orbit coupling $\lambda\, \boldsymbol{l} \cdot \boldsymbol{s}$ and tetragonal crystal field $\Delta(l_z^2 - \frac{2}{3})$ with $\xi = 2\lambda = 145$ meV fixed. **b,** Splitting of $T_{a/b}$ doublet under orthorhombic crystal field $\frac{1}{2}\Delta_{\rm ort}(n_{az} - n_{bz})$ at $\Delta = 250$ meV.

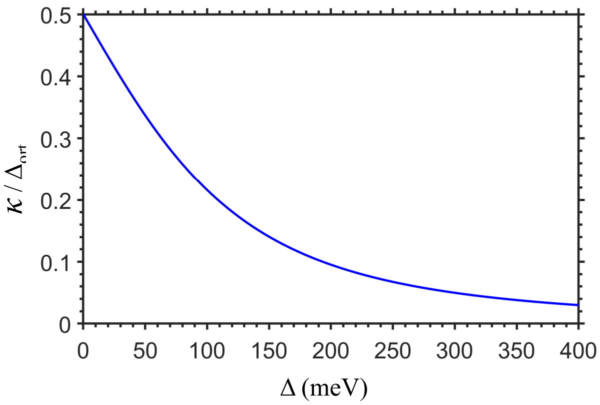


**Supplementary Figure 11**. In plane single-ion anisotropy parameter $\kappa$ in units of $\Delta_{\rm ort}$ as a function of $\Delta$ calculated with fixed $\xi = 2\lambda = 145$ meV.

### B. Interlayer coupling and magnetic phase transition

Owing to the orthorhombicity ($a < b$), the interlayer coupling $J_c^{(a)}$ within the $ac$-plane is stronger than $J_c^{(b)}$ in the $bc$-plane, i.e. $J_c^{(a/b)} = J_c(1 \pm \epsilon)$ with $\epsilon$ being a small positive number. At finite $\epsilon$, tetragonal symmetry of the interlayer interactions is broken. This partially relieves magnetic frustration caused by the body-centered interlayer stacking, and the sign of $J_c$ decides whether the magnetic structure is A-centered ($J_c > 0$) or B-centered ($J_c < 0$), see Supplementary Fig. 12. We explain the strain-induced magnetic phase transition as a consequence of reduction of tetragonal crystal field $\Delta$ which modifies pseudospin wave functions hence exchange coupling $J_c$ . Fig. 5 in the main text illustrates the interlayer exchange processes: (i) at large $\Delta$, the hole density of $xy$ orbital $n_{xy} \sim 0$ and the spin exchange between $az$-holes leads to AFM interaction; (ii) at small $\Delta$ with finite occupation of $xy$-hole, the exchange processes give rise to FM interaction due to Hund's coupling $J_H$. The reduction of tetragonal crystal field, which enlarges the hole density of $n_{xy}$ as shown in Supplementary Fig. 13a, decides the sign of $J_c$ and thus causes the magnetic transition from A- to B-centered structure.

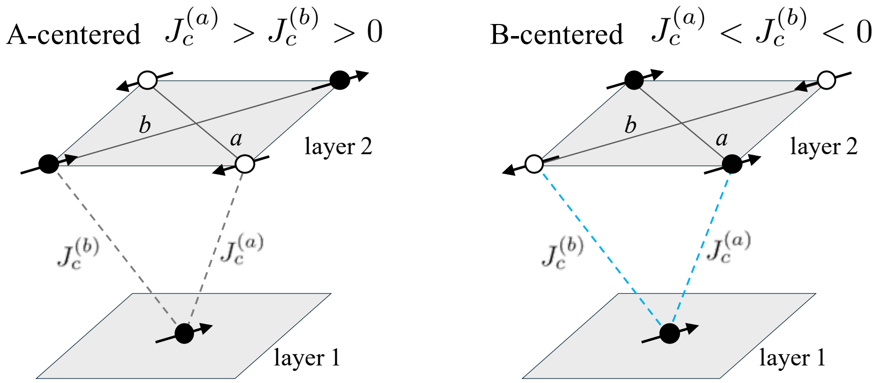


**Supplementary Figure 12**. **Sketches of the interlayer coupling for A- and B-centered magnetic structures.** Solid and empty balls indicates the Ru ions with anti-parallel aligned pseudospins (arrows). Layer1 and 2 are neighboring $RuO_2$ planes. The interlayer coupling between Ru ions are indicated with dashed lines, black (blue) for AFM (FM) interaction.

Collecting the above two contributions, the interlayer spin-orbital exchange Hamiltonian is obtained as:

$$\mathcal{H}_c^{ij} = \left( \frac{t_c^{'2}}{U} \hat{O}_{az}^{ij} + \frac{t_c^2}{U} \hat{O}_{xy}^{ij} \right) \boldsymbol{s}_i \cdot \boldsymbol{s}_j \ , \tag{S9}$$

where $t_c^{'}$ and $t_c$ are interlayer hoppings involving $az$ and $xy$ orbitals, respectively, and $U$ is the onsite Coulomb interaction.

The orbital operators are expressed as follows:

$$\hat{O}_{az}^{ij} = \left(1 + \frac{2\eta}{1-3\eta}\right) \hat{n}_{i,az}\hat{n}_{j,az} - \frac{\eta}{1-3\eta}(\hat{n}_{i,az} + \hat{n}_{j,az}) \ ,$$
$$\hat{O}_{xy}^{ij} = \left(1 + \frac{2\eta}{1-3\eta}\right) \hat{n}_{i,xy}\hat{n}_{j,xy} - \frac{\eta}{1-3\eta}(\hat{n}_{i,xy} + \hat{n}_{j,xy}) \ , \tag{S10}$$

where $\eta = J_H/U$, $\hat{n}_{xy}$ and $\hat{n}_{az}$ are hole density operators. They obey a local constraint $\hat{n}_{i,xy} + \hat{n}_{i,az} + \hat{n}_{i,bz} = 2$. The tetragonal crystal field $\Delta$ determines the hole densities $n_{xy}$ and $n_{az}$, and thus can manipulate the interlayer couplings.

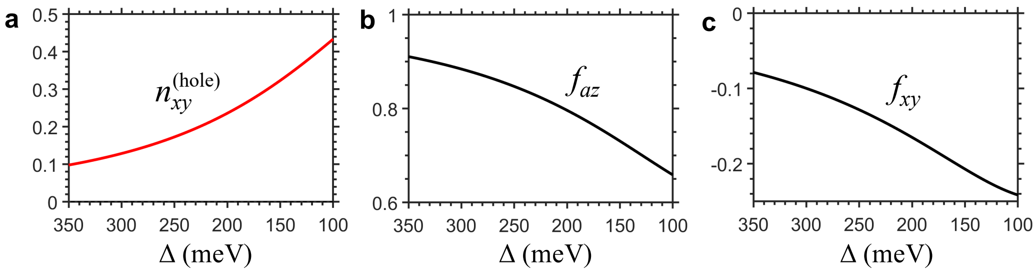


**Supplementary Figure 13**. **a**, Hole density $n_{xy}$ on $xy$ orbital as a function of tetragonal crystal field $\Delta$. **b-c**, Parameters $f_{az}$ and $f_{xy}$ defined in equation (S12) as a function of tetragonal crystal field $\Delta$, calculated with $\eta = 0.25$.

Projecting the spin-orbital Hamiltonian $\mathcal{H}_c$ (equation (S9)) onto the pseudospin $S = 1$ subspace, we get the interlayer exchange Hamiltonian $\mathcal{H}_c = J_c \, \boldsymbol{S}_i \cdot \boldsymbol{S}_j$ with

$$J_c = \frac{t_c^{'2}}{U} f_{az} + \frac{t_c^2}{U} f_{xy} \ . \tag{S11}$$

The parameters are:

$$f_{az} = \frac{\alpha^2}{2}\left(1 + \frac{2\eta}{1-3\eta}\right) + \alpha\beta + \beta^2 \ ,$$
$$f_{xy} = \alpha\left(\alpha - \frac{2\eta}{1-3\eta}\beta\right) \ , \tag{S12}$$

where $\alpha = \frac{1}{\sqrt{2}}\sin\theta_0 \sin\theta_1$ and $\beta = \cos\theta_0 \cos\theta_1$ are functions of angles $\theta_0$ and $\theta_1$ from equation (S5).

Supplementary Fig. 13b-c shows that the parameters $f_{az}$ and $f_{xy}$ have opposite signs and strongly depend on the tetragonal field $\Delta$. Therefore, the applied strain may tip the balance between AFM and FM contributions to the interlayer coupling $J_c$ in equation (S11). For $t_c = 2.4\ t'_c$, a sign change of $J_c$ occurs at $\Delta \sim 230$ meV as shown in Fig. 5 in the main text, which leads to the magnetic phase transition from A- to B-centered structure.

---


[1] Zhang, J. *et al.* Nano-resolved current-induced insulator-metal transition in the mott insulator $Ca_2RuO_4$. *Phys. Rev. X* **9**, 011032 (2019). URL https://link.aps.org/doi/10.1103/PhysRevX.9.011032.

[2] Braden, M., André, G., Nakatsuji, S. & Maeno, Y. Crystal and magnetic structure of $Ca_2RuO_4$: Magnetoelastic coupling and the metal-insulator transition. *Phys. Rev. B* **58**, 847–861 (1998). URL https://link.aps.org/doi/10.1103/PhysRevB.58.847.

[3] Chi, S., Ye, F., Cao, G., Cao, H. & Fernandez-Baca, J. A. Competition of three-dimensional magnetic phases in $Ca_2Ru_{1-x}Fe_xO_4$: A structural perspective. *Phys. Rev. B* **102**, 014452 (2020). URL https://link.aps.org/doi/10.1103/PhysRevB.102.014452.

[4] Pincini, D. *et al.* Persistence of antiferromagnetic order upon la substitution in the $4d^4$ mott insulator $Ca_2RuO_4$. *Phys. Rev. B* **98**, 014429 (2018). URL https://link.aps.org/doi/10.1103/PhysRevB.98.014429.

[5] Friedt, O. *et al.* Structural and magnetic aspects of the metal-insulator transition in $Ca_{2-x}Sr_xRuO_4$. *Phys. Rev. B* **63**, 174432 (2001). URL https://link.aps.org/doi/10.1103/PhysRevB.63.174432.

[6] Porter, D. G. *et al.* Guiding antiferromagnetic transitions in $Ca_2RuO_4$. *Sci. Rep.* **12**, 10957 (2022). URL https://doi.org/10.1038/s41598-022-14932-1.

[7] Steffens, P. *et al.* High-pressure diffraction studies on $Ca_2RuO_4$. *Phys. Rev. B* **72**, 094104 (2005). URL https://link.aps.org/doi/10.1103/PhysRevB.72.094104.
